# Supplementary material for: Band gap tuning by structural phase transition in Sm-substituted BiFeO3 powders
Source: arXiv:2504.08093 source file (2025-04-10)
Supplement: Supplementary file 1 [file 20250410_CHill_Supplm.pdf]

# Band gap tuning by structural phase transition in Sm-substituted $BiFeO_3$ powders – Supplementary information

Christina Hill,[1,2] Michele Melchiorre,[1] Cosme Milesi-Brault,[3] Pascale Gemeiner,[3] Fabienne Karolak,[3] Christine Bogicevic,[3] Brahim Dkhil,[3] Ingrid Cañero-Infante,[4] and Mael Guennou[1,2]

[1]*Department of Physics and Materials Science, University of Luxembourg, 41 rue du Brill, 4422 Belvaux, Luxembourg*
[2]*Inter-institutional Research Group Uni.lu–LIST on Ferroic Materials, 41 rue du Brill, 4422 Belvaux, Luxembourg*
[3]*Université Paris-Saclay, CNRS, CentraleSupélec, Laboratoire SPMS, 91190 Gif-sur-Yvette, France*
[4]*Université de Lyon, Institut des Nanotechnologies de Lyon, CNRS UMR 5270 ECL INSA UCBL CPE, 1 rue Enrico Fermi, F-69621 Villeurbanne, France*

## CONTENTS

I. Grain size and morphology (SEM analysis) 2
II. XRD patterns at room temperature 3
III. Composition-dependent Raman analysis 4
IV. Composition-dependent diffuse reflectance measurements 5
V. Absorption as a function of temperature for different compositions 6
VI. Temperature-dependent XRD analysis for Sm concentration of 14% 7
References 8

## I. GRAIN SIZE AND MORPHOLOGY (SEM ANALYSIS)

All powders showed comparable grain distribution and morphology. As an example, we show the SEM image of the powder with 18% Samarium concentration in Fig. S1. The individual grains have a faceted shape and an average size of of 370 nm.

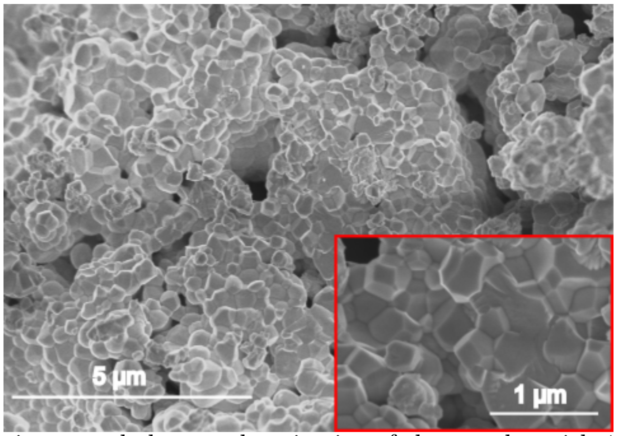


Figure S1: SEM picture showing morphology and grain size of the powder with 18% Samarium concentration.

The average grain sizes for all other powders were similarly determined and are summarized in the Table below. They are all well above the value for which significant size effects on the absorption properties have been reported [1].

Table SI: Average grain size for all powders.

| Sample | Average grain size |
|---|---|
| Sm 10% | 370 nm |
| Sm 12% | 520 nm |
| Sm 14% | 400 nm |
| Sm 16% | 370 nm |
| Sm 18% | 370 nm |
| Sm 20% | 430 nm |

## II. XRD PATTERNS AT ROOM TEMPERATURE

Fig. S2 shows the XRD patterns of the pellets for all compositions measured at room temperature. The peak assignment clearly shows that the crystal structure is dominated by the rhombohedral $R3c$ phase for Sm content of 10% and 12% and by the $Pnma$ phase for 20% Sm. In the intermediate range of Sm concentrations (14% and 16% and 18%), we see a coexistence of the two phases. Weak peaks between 26° and 31° are visible could be associated to $Bi_2Fe_4O_9$, as previously reported [2, 3]. The (112) reflection of the PZO-like $Pbam$ phase would also fall in this range[2, 4, 5]. In both cases, the very small amount is not expected to affect the conclusions of the paper.

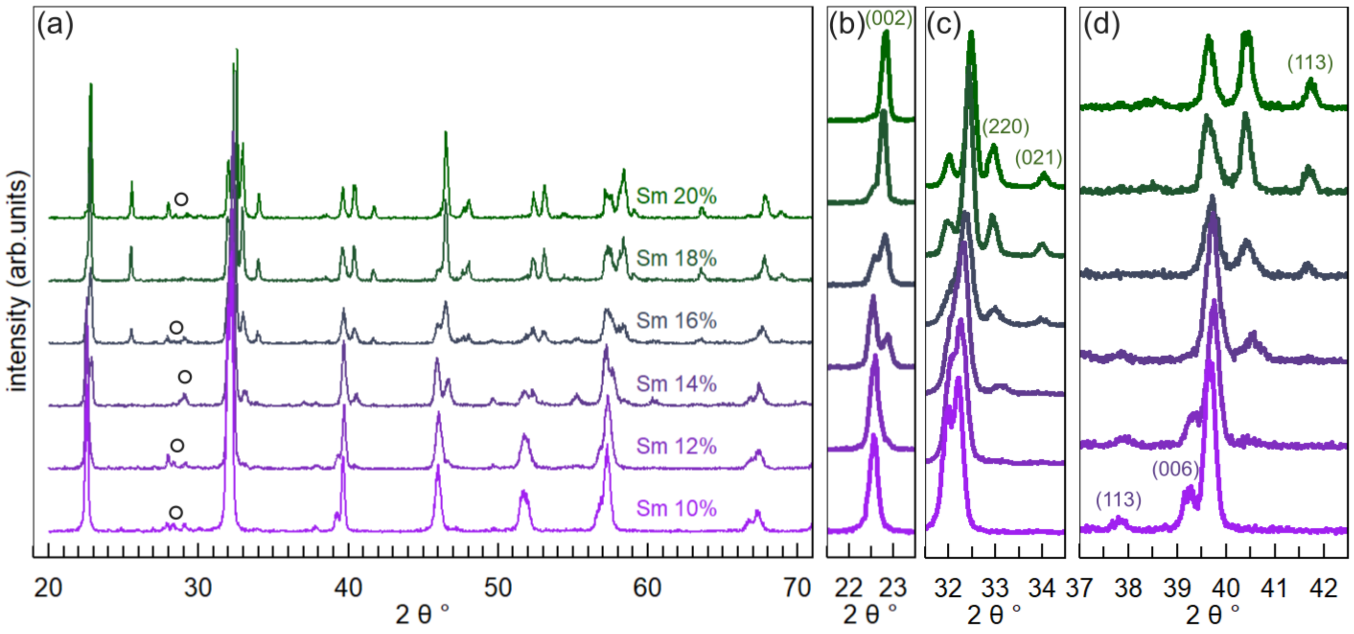


Figure S2: XRD patterns measured on pellets at room temperature. Peaks indicated by black circles could originate from a minute fraction of a $Bi_2Fe_4O_9$ impurity phase or a $Pbam$ phase. (b)-(d) show zooms on the most relevant peaks, with indexing corresponding to the $Pnma$ phase (top) and the $R3c$ phase (bottom).

## III. COMPOSITION-DEPENDENT RAMAN ANALYSIS

The Raman spectra of the powders for all compositions are shown in Fig. S3. For the Sm content of 10% and 12%, the Raman spectrum is essentially similar to the spectrum known for pure $BiFeO_3$, consistent with the expectation from the phase diagram [6, 7] and the XRD measurements above. For 20% Sm, the spectrum is radically different with notably the presence of a characteristic peak at 400 $cm^{-1}$; it can be associated to the pure *Pnma* phase. Intermediate compositions have a spectrum that shows a mixture of both spectra to various degrees. Phase coexistence is most proncounced for 14% and is barely visible for 18%. No sign of an additional phase can be detected.

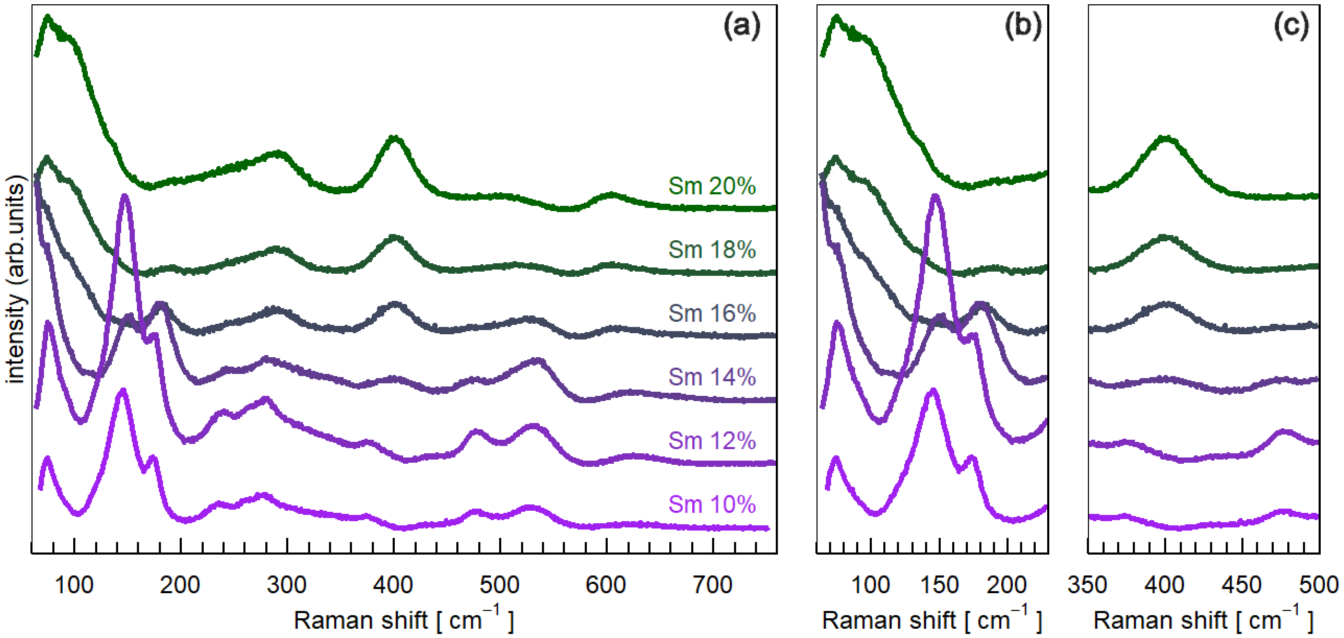


Figure S3: Composition dependent Raman spectra measured at room temperature with a 633 nm excitation (a) Full frequency range, (b) prominent double peak of the *R*3*c* phase in the low frequency range and (c) distinctive high intensity peak at 400 $cm^{-1}$ for the non-polar *Pnma* phase at high Sm concentrations.

## IV. COMPOSITION-DEPENDENT DIFFUSE REFLECTANCE MEASUREMENTS

Fig. S4 shows the diffuse reflectance measured at room temperature for Samarium concentrations from 10% to 20%. The absorption spectra are calculated from the diffuse reflectance using the Kubelka-Munk function $F(R)$.

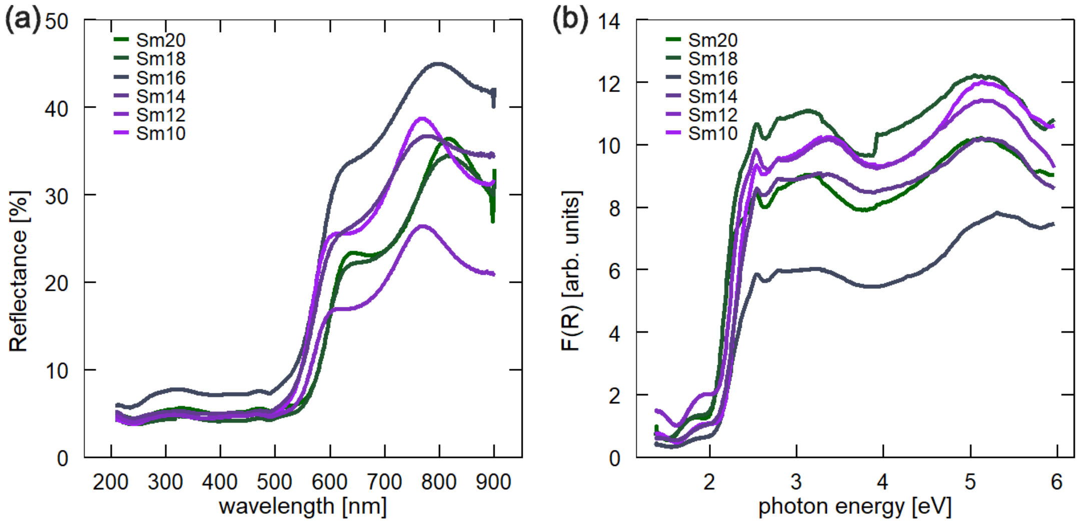


Figure S4: (a) Diffuse Reflectance measured at room temperature for different Samarium concentrations ranging from 10% to 20%. (b) Absorption spectra derived from the diffuse reflectance using Kubelka-Munk functions $F(R)$.

## V. ABSORPTION AS A FUNCTION OF TEMPERATURE FOR DIFFERENT COMPOSITIONS

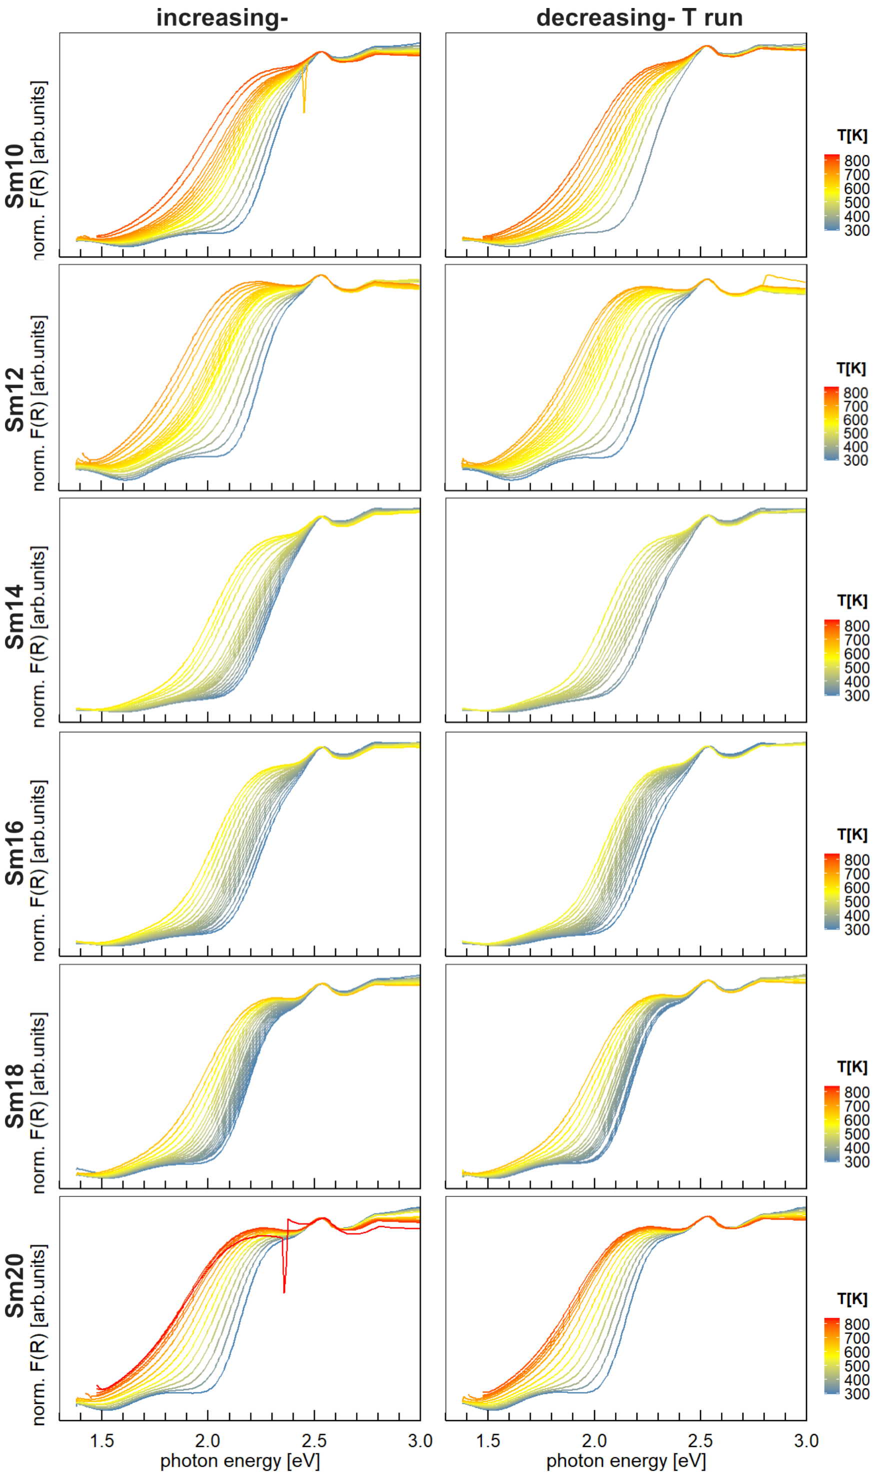


Figure S5: Absorption spectra derived from the diffuse reflectance using Kubelka-Munk functions F(R) for increasing- and decreasing- temperature run for all compositions. Spectra are normalized to the peak around 2.5 eV.

## VI. TEMPERATURE-DEPENDENT XRD ANALYSIS FOR SM CONCENTRATION OF 14%

Fig. S6 shows the XRD pattern for the Sm concentration of 14% for the increasing- and decreasing-temperature run. The spectra are stacked vertically, starting with the increasing temperature run at the bottom. The indexing for the two phases are indicated.

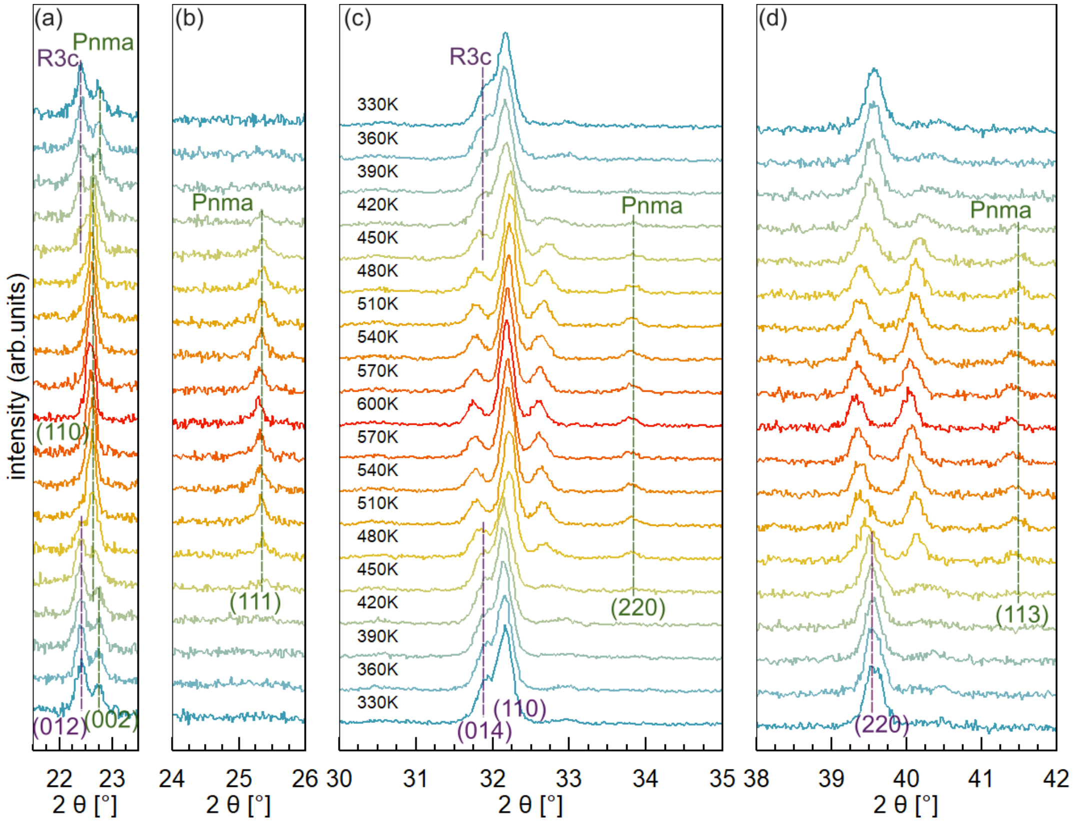


Figure S6: XRD pattern for 14% Sm concentration for the increasing and the decreasing temperature run. The spectra are stacked vertically, starting with the increasing temperature run at the bottom. The distinctive reflections of the rhombohedral $R3c$ phase ad the orthorhombic $Pnma$ phase are indicated.

[1] X. Bai, J. Wei, B. Tian, Y. Liu, T. Reiss, N. Guiblin, P. Gemeiner, B. Dkhil, and I. C. Infante, Size Effect on Optical and Photocatalytic Properties in $BiFeO_3$ Nanoparticles, The Journal of Physical Chemistry C **120**, 3595 (2016).

[2] F. F. Orudzhev, N. M.-R. Alikhanov, S. M. Ramazanov, D. S. Sobola, R. K. Murtazali, E. H. Ismailov, R. D. Gasimov, A. S. Aliev, and Ş. Ţălu, Morphotropic phase boundary enhanced photocatalysis in sm doped $BiFeO_3$, Molecules **27**, 7029 (2022).

[3] J. Bielecki, P. Svedlindh, D. T. Tibebu, S. Cai, S.-G. Eriksson, L. Börjesson, and C. S. Knee, Structural and magnetic properties of isovalently substituted multiferroic $BiFeO_3$: Insights from raman spectroscopy, Physical Review B **86**, 184422 (2012).

[4] A. Pakalniškis, R. Skaudžius, D. V. Zhaludkevich, S. I. Latushka, V. Sikolenko, A. V. Sysa, M. Silibin, K. Mažeika, D. Baltrūnas, G. Niaura, M. Talaikis, D. V. Karpinsky, and A. Kareiva, Pressure induced phase transitions in sm-doped $BiFeO_3$ in the morphotropic phase boundary, Materials Chemistry and Physics **277**, 125458 (2022).

[5] X. X. Shi, X. Q. Liu, and X. M. Chen, Structure evolution and piezoelectric properties across the morphotropic phase boundary of sm-substituted $BiFeO_3$ ceramics, Journal of Applied Physics **119**, 064104 (2016).

[6] D. Kan, C.-J. Cheng, V. Nagarajan, and I. Takeuchi, Composition and temperature-induced structural evolution in La, Sm, and Dy substituted $BiFeO_3$ epitaxial thin films at morphotropic phase boundaries, Journal of Applied Physics **110**, 014106 (2011).

[7] F. Mumtaz, S. Nasir, G. Jaffari, and S. Shah, Chemical pressure exerted by rare earth substitution in $BiFeO_3$: Effect on crystal symmetry, band structure and magnetism, Journal of Alloys and Compounds **876**, 160178 (2021).
